# Supplementary material for: Explainable classification of astronomical uncertain time series
Source: arXiv:2210.00869 source file (2026-03-09)
Supplement: Supplementary file 1 [file uSAST_PLAsTiCC_supplementary.pdf]

---

# EXPLAINABLE CLASSIFICATION OF ASTRONOMICAL UNCERTAIN TIME SERIES

(SUPPLEMENTARY MATERIAL)

---

**Michael Franklin MBOUOPDA**

LIMOS

University Clermont Auvergne  
Clermont-Ferrand

michael.mbouopda@uca.fr

**Emille E. O. ISHIDA**

Laboratory of Physics of Clermont

University Clermont Auvergne  
Clermont-Ferrand

emille.ishida@clermont.in2p3.fr

**Engelbert MEPHU NGUIFO**

LIMOS

University Clermont Auvergne  
Clermont-Ferrand

engelbert.mephu\_nguifo@uca.fr

**Emmanuel GANGLER**

Laboratory of Physics of Clermont

University Clermont Auvergne  
Clermont-Ferrand

emmanuel.gangler@clermont.in2p3.fr

## 1 SAST-based methods results

Table 1: SAST<X> models results on the PLAsTiCC dataset average over 3 runs. The starred row is the run that achieved the lowest cross entropy loss.

|             | Classifier | Precision       | Recall          | F1 score        | LogLoss         | Time (h)          |
|-------------|------------|-----------------|-----------------|-----------------|-----------------|-------------------|
| [c]4*SAST   | RF         | $0.59 \pm 0.04$ | $0.61 \pm 0.00$ | $0.56 \pm 0.01$ | $1.29 \pm 0.05$ | $16.41 \pm 0.52$  |
|             | RidgeCV    | $0.56 \pm 0.00$ | $0.57 \pm 0.00$ | $0.55 \pm 0.00$ | $2.22 \pm 0.01$ | $16.41 \pm 0.52$  |
|             | XGBoost    | $0.65 \pm 0.01$ | $0.67 \pm 0.00$ | $0.63 \pm 0.00$ | $1.16 \pm 0.01$ | $16.41 \pm 0.52$  |
|             | XGBoost*   | 0.65            | 0.67            | 0.64            | 1.15            | 16.23             |
| [c]4*SASTd  | RF         | $0.58 \pm 0.05$ | $0.60 \pm 0.00$ | $0.54 \pm 0.00$ | $1.33 \pm 0.08$ | $12.79 \pm 0.84$  |
|             | RidgeCV    | $0.56 \pm 0.01$ | $0.58 \pm 0.01$ | $0.55 \pm 0.01$ | $2.20 \pm 0.00$ | $12.79 \pm 0.84$  |
|             | XGBoost    | $0.66 \pm 0.02$ | $0.68 \pm 0.00$ | $0.64 \pm 0.00$ | $1.14 \pm 0.00$ | $12.79 \pm 0.841$ |
|             | XGBoost*   | 0.66            | 0.68            | 0.64            | 1.13            | 11.84             |
| [c]4*SASTdc | RF         | $0.58 \pm 0.03$ | $0.61 \pm 0.00$ | $0.55 \pm 0.00$ | $1.33 \pm 0.04$ | $12.99 \pm 0.30$  |
|             | RidgeCV    | $0.52 \pm 0.02$ | $0.54 \pm 0.01$ | $0.52 \pm 0.01$ | $2.25 \pm 0.00$ | $12.99 \pm 0.30$  |
|             | XGBoost    | $0.66 \pm 0.01$ | $0.68 \pm 0.00$ | $0.64 \pm 0.01$ | $1.14 \pm 0.01$ | $12.99 \pm 0.30$  |
|             | XGBoost*   | 0.65            | 0.68            | 0.64            | 1.14            | 13.04             |

## 2 uSAST-based methods results

Table 2: uSAST<X> models results on the PLAsTiCC dataset average over 3 runs. The row with the star is the run that achieved the lowest cross entropy loss. Subsequence length: from 16 to 32 with a step of 1.

|              | Classifier | Precision       | Recall          | F1 score        | LogLoss         | Time (h)         |
|--------------|------------|-----------------|-----------------|-----------------|-----------------|------------------|
| [c]5*uSAST   | RF         | $0.62 \pm 0.01$ | $0.66 \pm 0.01$ | $0.60 \pm 0.01$ | $1.20 \pm 0.03$ | $53.61 \pm 0.10$ |
|              | RidgeCV    | $0.33 \pm 0.02$ | $0.34 \pm 0.02$ | $0.33 \pm 0.02$ | $2.98 \pm 0.11$ | $53.61 \pm 0.10$ |
|              | XGBoost    | $0.69 \pm 0.00$ | $0.70 \pm 0.00$ | $0.66 \pm 0.00$ | $1.04 \pm 0.01$ | $53.61 \pm 0.10$ |
|              | XGBoost*   | 0.69            | 0.70            | 0.66            | 1.04            | 53.56            |
| [c]5*uSASTd  | RF         | $0.61 \pm 0.03$ | $0.64 \pm 0.00$ | $0.58 \pm 0.00$ | $1.20 \pm 0.04$ | $41.58 \pm 0.47$ |
|              | RidgeCV    | $0.35 \pm 0.01$ | $0.37 \pm 0.01$ | $0.35 \pm 0.01$ | $2.90 \pm 0.06$ | $41.58 \pm 0.47$ |
|              | XGBoost    | $0.70 \pm 0.01$ | $0.70 \pm 0.00$ | $0.67 \pm 0.00$ | $1.06 \pm 0.02$ | $41.58 \pm 0.47$ |
|              | XGBoost*   | 0.71            | 0.70            | 0.67            | 1.04            | 41.78            |
| [c]5*uSASTdc | RF         | $0.60 \pm 0.00$ | $0.64 \pm 0.01$ | $0.58 \pm 0.00$ | $1.21 \pm 0.00$ | $40.45 \pm 1.00$ |
|              | RidgeCV    | $0.37 \pm 0.04$ | $0.38 \pm 0.03$ | $0.37 \pm 0.03$ | $2.78 \pm 0.07$ | $40.45 \pm 1.00$ |
|              | XGBoost    | $0.69 \pm 0.01$ | $0.70 \pm 0.00$ | $0.66 \pm 0.00$ | $1.04 \pm 0.02$ | $40.45 \pm 1.00$ |
|              | XGBoost*   | 0.68            | 0.70            | 0.66            | 1.03            | 41.16            |

Table 3: uSAST<X> models results on the PLAsTiCC dataset average over 3 runs. The row with the star is the run that achieved the lowest cross entropy loss. Subsequence length: from 20 to 60 with a step of 10.

|              | Classifier | Precision       | Recall          | F1 score        | LogLoss         | Time (h)         |
|--------------|------------|-----------------|-----------------|-----------------|-----------------|------------------|
| [c]5*uSAST   | RF         | $0.64 \pm 0.01$ | $0.68 \pm 0.01$ | $0.62 \pm 0.01$ | $1.09 \pm 0.01$ | $51.03 \pm 0.12$ |
|              | Ridge      | $0.39 \pm 0.01$ | $0.40 \pm 0.01$ | $0.39 \pm 0.01$ | $2.82 \pm 0.08$ | $51.03 \pm 0.12$ |
|              | XGBoost    | $0.72 \pm 0.01$ | $0.72 \pm 0.00$ | $0.69 \pm 0.01$ | $0.96 \pm 0.01$ | $51.03 \pm 0.12$ |
|              | XGBoost*   | 0.71            | 0.72            | 0.69            | 0.95            | 51.17            |
| [c]5*uSASTd  | RF         | $0.65 \pm 0.02$ | $0.67 \pm 0.01$ | $0.62 \pm 0.01$ | $1.12 \pm 0.04$ | $43.49 \pm 0.27$ |
|              | Ridge      | $0.39 \pm 0.02$ | $0.41 \pm 0.02$ | $0.40 \pm 0.02$ | $2.77 \pm 0.07$ | $43.49 \pm 0.27$ |
|              | XGBoost    | $0.72 \pm 0.00$ | $0.73 \pm 0.00$ | $0.70 \pm 0.01$ | $0.97 \pm 0.01$ | $43.49 \pm 0.27$ |
|              | XGBoost*   | 0.72            | 0.73            | 0.69            | 0.95            | 43.18            |
| [c]5*uSASTdc | RF         | $0.67 \pm 0.03$ | $0.67 \pm 0.00$ | $0.62 \pm 0.00$ | $1.11 \pm 0.00$ | $43.52 \pm 0.72$ |
|              | Ridge      | $0.39 \pm 0.02$ | $0.40 \pm 0.02$ | $0.39 \pm 0.02$ | $2.79 \pm 0.02$ | $43.52 \pm 0.72$ |
|              | XGBoost    | $0.71 \pm 0.01$ | $0.72 \pm 0.01$ | $0.69 \pm 0.01$ | $0.96 \pm 0.01$ | $43.52 \pm 0.72$ |
|              | XGBoost*   | 0.70            | 0.72            | 0.68            | 0.95            | 44.26            |

3 Results of state-of-the-art models

Table 4: Performance of state-of-the-art models average over 3 runs. MUSE uses a linear classifier. The row with the star is the run that achieved the lowest cross entropy loss

|             | Classifier | Precision       | Recall          | F1 score        | LogLoss         | Time (h)        |
|-------------|------------|-----------------|-----------------|-----------------|-----------------|-----------------|
| MUSE        | -          | $0.71 \pm 0.01$ | $0.73 \pm 0.01$ | $0.71 \pm 0.01$ | $1.78 \pm 0.03$ | $3.36 \pm 0.04$ |
| [c]4*ROCKET | RF         | $0.75 \pm 0.01$ | $0.75 \pm 0.00$ | $0.72 \pm 0.00$ | $0.94 \pm 0.03$ | $0.05 \pm 0.00$ |
|             | Ridge      | $0.71 \pm 0.01$ | $0.71 \pm 0.01$ | $0.70 \pm 0.01$ | $2.07 \pm 0.00$ | $0.05 \pm 0.00$ |
|             | XGBoost    | $0.77 \pm 0.00$ | $0.77 \pm 0.00$ | $0.75 \pm 0.00$ | $0.82 \pm 0.01$ | $0.05 \pm 00$   |
|             | XGBoost*   | 0.78            | 0.77            | 0.75            | 0.81            | 0.05            |
